# Supplementary material for: Communication-Efficient Federated Learning via Predictive Coding
Source: arXiv:2108.00918 source file (2022-01-09)
Supplement: Supplementary file 1 [file bios.tex]

\vskip 0pt plus -1fil

\begin{IEEEbiography}[{\includegraphics[width=1in,height=1.25in,clip]{bio_photos/kai Yue.png}}]{Kai Yue}
(Graduate Student Member, IEEE) received his B.E. degree (with honors) in electronic and information engineering from the University of Science and Technology of China, Hefei, China, in 2020.
He is currently working toward the Ph.D. degree in Electrical Engineering at the North Carolina State University. 
His research interests include federated learning, image processing, and video coding.     
\end{IEEEbiography}

\vskip 0pt plus -1fil
\begin{IEEEbiography}[{\includegraphics[width=1in,height=1.25in,clip]{bio_photos/Richeng Jin.jpg}}]{Richeng Jin}
(Member, IEEE) received the B.S. degree in information and communication engineering from Zhejiang University, Hangzhou, China, in 2015, and the Ph.D. degree in electrical engineering from the North Carolina State University, Raleigh, NC, USA, in 2020.
He is currently a Postdoctoral Researcher in the Department of Electrical and Computer Engineering at the North Carolina State University, Raleigh, NC, USA. 
His current research interests are in the areas of game theory, wireless security and privacy, and machine learning.
\end{IEEEbiography}

\vskip 0pt plus -1fil
\begin{IEEEbiography}[{\includegraphics[width=1in,height=1.25in,clip]{bio_photos/ChauWaiWong.jpg}}]{Chau-Wai Wong}
(Member, IEEE) received his B.Eng. and M.Phil. degrees in electronic and information engineering from The Hong Kong Polytechnic University, in 2008 and 2010, and the Ph.D. degree in electrical engineering from the University of Maryland, College Park, MD, USA, in 2017. 
He is currently an Assistant Professor with the Department of Electrical and Computer Engineering, the Forensic Sciences Cluster, and the Secure Computing Institute, North Carolina State University. 
He was a data scientist at Origin Wireless, Inc., Greenbelt, MD, USA. His research interests include multimedia forensics, statistical signal processing, machine learning, data analytics, and video coding. 
Dr. Wong received a Top-Four Student Paper Award, Future Faculty Fellowship, HSBC Scholarship, and Hitachi Scholarship. 
He was the General Secretary of the IEEE PolyU Student Branch from 2006 to 2007. 
He was involved in organizing the third edition of the IEEE Signal Processing Cup in 2016 on electric network frequency forensics.
\end{IEEEbiography}

\vskip 0pt plus -1fil
\begin{IEEEbiography}[{\includegraphics[width=1in,height=1.25in,clip]{bio_photos/Huaiyu Dai-IEEE.png}}]{Huaiyu Dai}
(Fellow, IEEE) received the B.E. and M.S. degrees in electrical engineering from Tsinghua University, Beijing, China, in 1996 and 1998, respectively, and the Ph.D. degree in electrical engineering from Princeton University, Princeton, NJ in 2002. 
    
He was with Bell Labs, Lucent Technologies, Holmdel, NJ, in summer 2000, and with AT\&T Labs-Research, Middletown, NJ, in summer 2001. He is currently a Professor of Electrical and Computer Engineering with NC State University, Raleigh, holding the title of University Faculty Scholar. His research interests are in the general areas of communications, signal processing, networking, and computing. His current research focuses on machine learning and artificial intelligence for communications and networking, multilayer and interdependent networks, dynamic spectrum access and sharing, as well as security and privacy issues in the above systems.
    
He has served as an editor for IEEE Transactions on Communications, IEEE Transactions on Signal Processing, and IEEE Transactions on Wireless Communications. Currently he is an Area Editor in charge of wireless communications for IEEE Transactions on Communications, and a member of the Executive Editorial Committee for IEEE Transactions on Wireless Communications. He was a co-recipient of best paper awards at 2010 IEEE International Conference on Mobile Ad-hoc and Sensor Systems (MASS 2010), 2016 IEEE INFOCOM BIGSECURITY Workshop, and 2017 IEEE International Conference on Communications (ICC 2017).
\end{IEEEbiography}
